# Supplementary material for: CHiSafetyBench: A Chinese Hierarchical Safety Benchmark for Large Language Models
Source: arXiv:2406.10311 source file (2024-09-02)
Supplement: Supplementary file 1 [file checklist.tex]

\section{Reproducibility Checklist}
\subsection{This paper:}

\begin{itemize}
\item Includes a conceptual outline and/or pseudocode description of AI methods introduced (yes)
\item Clearly delineates statements that are opinions, hypothesis, and speculation from objective facts and results (yes)
\item Provides well marked pedagogical references for less-familiare readers to gain background necessary to replicate the paper (yes)
\end{itemize}

\subsection{Does this paper make theoretical contributions? (no)}

% If yes, please complete the list below.
% \begin{itemize}
% \item All assumptions and restrictions are stated clearly and formally. (yes/partial/no)
% \item All novel claims are stated formally (e.g., in theorem statements). (yes/partial/no)
% \item Proofs of all novel claims are included. (yes/partial/no)
% \item Proof sketches or intuitions are given for complex and/or novel results. (yes/partial/no)
% \item Appropriate citations to theoretical tools used are given. (yes/partial/no)
% \item All theoretical claims are demonstrated empirically to hold. (yes/partial/no/NA)
% \item All experimental code used to eliminate or disprove claims is included. (yes/no/NA)
% \end{itemize}


% 如果是，请完成下面的列表。

% 给出了在所选数据集上进行实验的动机（是/部分/否/NA）
% 本文介绍的所有新数据集均包含在数据附录中。（是/部分/否/NA）
% 本文介绍的所有新数据集将在论文发表后公开，并提供许可证，允许免费用于研究目的。（是/部分/否/NA）
% 从现有文献中提取的所有数据集（可能包括作者自己之前发表的作品）都附有适当的引文。（是/否/NA）
% 从现有文献中提取的所有数据集（可能包括作者自己之前发表的作品）都是公开的。（是/部分/否/NA）
% 所有未公开的数据集都进行了详细描述，并解释了为什么公开的替代方案在科学上不能令人满意。（是/部分/否/NA）



\subsection{Does this paper rely on one or more datasets? (yes)}

If yes, please complete the list below.
\begin{itemize}
\item A motivation is given for why the experiments are conducted on the selected datasets (yes)
\item All novel datasets introduced in this paper are included in a data appendix. (no)
\item All novel datasets introduced in this paper will be made publicly available upon publication of the paper with a license that allows free usage for research purposes. (yes)
\item All datasets drawn from the existing literature (potentially including authors’ own previously published work) are accompanied by appropriate citations. (yes)
\item All datasets drawn from the existing literature (potentially including authors’ own previously published work) are publicly available. (yes)
\item All datasets that are not publicly available are described in detail, with explanation why publicly available alternatives are not scientifically satisficing. (NA)
\end{itemize}


% 这篇论文是否包括计算实验？（是/否）
% 如果是，请完成下面的列表。

% 附录中包含了预处理数据所需的任何代码。（是/部分/否）。
% 进行和分析实验所需的所有源代码都包含在代码附录中。（是/部分/否）
% 进行和分析实验所需的所有源代码将在论文发表后公开，并附有允许免费用于研究目的的许可证。（是/部分/否）
% 所有实现新方法的源代码都有详细说明实现的注释，并引用了每个步骤所来自的论文（是）
% 如果算法依赖于随机性，则用于设置种子的方法的描述足以允许复制结果。（否）
% 本文指定了用于运行实验的计算基础设施（硬件和软件），包括 GPU/CPU 模型；内存量；操作系统；相关软件库和框架的名称和版本。（否）
% 本文正式描述了所使用的评估指标并解释了选择这些指标的动机。（是）
% 本文说明了计算每个报告结果所使用的算法运行次数。（否）
% 实验分析不仅限于单维的性能总结（例如平均值、中位数），还包括变化、置信度或其他分布信息的度量。（是）
% 使用适当的统计检验（例如 Wilcoxon 符号秩检验）来判断性能的任何改进或下降的重要性。（否）
% 本文列出了论文实验中每个模型/算法使用的所有最终（超）参数。（部分）
% 本文阐述了在论文开发过程中每个（超）参数尝试的值的数量和范围，以及用于选择最终参数设置的标准。（部分）


\subsection{Does this paper include computational experiments? (yes)}
If yes, please complete the list below.
\begin{itemize}
\item Any code required for pre-processing data is included in the appendix. (no).
\item All source code required for conducting and analyzing the experiments is included in a code appendix. (no)
\item All source code required for conducting and analyzing the experiments will be made publicly available upon publication of the paper with a license that allows free usage for research purposes. (yes)
\item All source code implementing new methods have comments detailing the implementation, with references to the paper where each step comes from (yes)
\item If an algorithm depends on randomness, then the method used for setting seeds is described in a way sufficient to allow replication of results. (yes)
\item This paper specifies the computing infrastructure used for running experiments (hardware and software), including GPU/CPU models; amount of memory; operating system; names and versions of relevant software libraries and frameworks. (no)
\item This paper formally describes evaluation metrics used and explains the motivation for choosing these metrics. (yes)
\item This paper states the number of algorithm runs used to compute each reported result. (no)
\item Analysis of experiments goes beyond single-dimensional summaries of performance (e.g., average; median) to include measures of variation, confidence, or other distributional information. (no)
\item The significance of any improvement or decrease in performance is judged using appropriate statistical tests (e.g., Wilcoxon signed-rank). (no)
\item This paper lists all final (hyper-)parameters used for each model/algorithm in the paper’s experiments. (NA)
\item This paper states the number and range of values tried per (hyper-) parameter during development of the paper, along with the criterion used for selecting the final parameter setting. (NA)
\end{itemize}
